# Supplementary material for: Coil Sketching for computationally-efficient MR iterative reconstruction
Source: arXiv:2305.06482 ancillary file (2023-10-11)
Supplement: Supplementary file 1 [file Supporting_Material.pdf]

# Supporting Material

## S1 Hessian sketch derivation

We start with Equation (6) in the manuscript.

$$\mathbf{u}^* = \operatorname*{argmin}_{\mathbf{u}\in\mathcal{C}} h(\mathbf{u}) := \|\mathbf{B}\mathbf{u} - \mathbf{v}\|_2^2 \tag{S1}$$

We define $\hat{h}(\mathbf{u}) \approx h(\mathbf{u})$, a second-order Taylor expansion of $h(\mathbf{u})$ around initial estimate $\mathbf{u}_0$.

$$\begin{aligned}\hat{h}(\mathbf{u}) = h(\mathbf{u}_0) &+ \frac{1}{1!}\nabla h(\mathbf{u}_0)^\mathsf{T}(\mathbf{u} - \mathbf{u}_0) \\ &+ \frac{1}{2!}(\mathbf{u} - \mathbf{u}_0)^\mathsf{T}\nabla^2 h(\mathbf{u})(\mathbf{u} - \mathbf{u}_0)\end{aligned} \tag{S2}$$

where $\nabla h(\mathbf{u})$ and $\nabla^2 h(\mathbf{u})$ are the gradient and hessian of $h(\mathbf{u})$ respectively.

$$\begin{aligned}\hat{h}(\mathbf{u}) &= h(\mathbf{u}_0) + \left(\mathbf{B}^\mathsf{T}(\mathbf{B}\mathbf{u}_0 - \mathbf{v})\right)^\mathsf{T}(\mathbf{u} - \mathbf{u}_0) \\ &\quad + \frac{1}{2}(\mathbf{u} - \mathbf{u}_0)^\mathsf{T}\mathbf{B}^\mathsf{T}\mathbf{B}(\mathbf{u} - \mathbf{u}_0) \\ &= h(\mathbf{u}_0) + \langle \mathbf{B}^\mathsf{T}(\mathbf{B}\mathbf{u}_0 - \mathbf{v}), \mathbf{u} - \mathbf{u}_0\rangle \\ &\quad + \frac{1}{2}\|\mathbf{B}(\mathbf{u} - \mathbf{u}_0)\|_2^2 \\ &= \frac{1}{2}\|\mathbf{B}(\mathbf{u} - \mathbf{u}_0)\|_2^2 + \langle \mathbf{u}, \mathbf{B}^\mathsf{T}(\mathbf{B}\mathbf{u}_0 - \mathbf{v})\rangle \\ &\quad + h(\mathbf{u}_0) - \langle \mathbf{B}^\mathsf{T}(\mathbf{B}\mathbf{u}_0 - \mathbf{v}), \mathbf{u}_0\rangle\end{aligned} \tag{S3}$$

We sketch the term that corresponds to the hessian of $h(\mathbf{u})$ and drop the terms that do not depend on $\mathbf{u}$.

$$h_\mathbf{S}(\mathbf{u}) = \frac{1}{2}\|\mathbf{S}\mathbf{B}(\mathbf{u} - \mathbf{u}_0)\|_2^2 + \langle \mathbf{u}, \mathbf{B}^\mathsf{T}(\mathbf{B}\mathbf{u}_0 - \mathbf{v})\rangle \tag{S4}$$

Finally, the iterative hessian sketch is defined below:

$$\begin{aligned}\mathbf{u}^{t+1} = \operatorname*{argmin}_{\mathbf{u}\in\mathcal{C}} h_\mathbf{S}^t(\mathbf{u}) := \frac{1}{2}&\|\mathbf{S}^t\mathbf{B}(\mathbf{u} - \mathbf{u}^t)\|_2^2 \\ &+ \langle \mathbf{u}, \mathbf{B}^\mathsf{T}(\mathbf{B}\mathbf{u}^t - \mathbf{v})\rangle\end{aligned} \tag{S5}$$

# S2 Solver implementation details

## S2.1 $\ell_2$-norm regularization

We consider the following optimization problem for image reconstruction:

$$\mathbf{x}^* = \underset{\mathbf{x}}{\operatorname{argmin}}\, \bar{f}(\mathbf{x}) + \bar{g}(\mathbf{x}), \tag{S6}$$

$$\bar{g}(\mathbf{x}) = \frac{\lambda}{2}\|\mathbf{x}\|_2^2, \tag{S7}$$

where $\bar{f} : \mathbb{C}^D \to \mathbb{R}$ is the data consistency function and $\bar{g} : \mathbb{C}^D \to \mathbb{R}$ is the regularization function. The data consistency function is a quadratic term in both conventional and sketched reconstruction. Therefore, we can express equation S6 as a linear equation $\bar{\mathbf{A}}\mathbf{x}^* = \bar{\mathbf{y}}$ and solve it efficiently with the Conjugate Gradient (CG) algorithm [32,33,34] shown in Algorithm S1. In general, this algorithm can solve linear equations of the form $\bar{\mathbf{A}}\mathbf{x}^* = \bar{\mathbf{y}}$ efficiently when matrix $\bar{\mathbf{A}}$ is symmetric and positive definite. In both conventional and sketched reconstruction, the respective matrix $\bar{\mathbf{A}}$ complies with this requirement.

**Algorithm S1** Conjugate Gradient

**Input**: Model matrix $\bar{\mathbf{A}}$, data vector $\bar{\mathbf{y}}$
**Output**: Reconstructed image $\mathbf{x}_K$
Initialize $\mathbf{x}_0$
$\mathbf{r}_0 = \bar{\mathbf{y}} - \bar{\mathbf{A}}\mathbf{x}_0$
$\mathbf{p}_0 = \mathbf{r}_0$
**for** $k = 0, ..., K-1$ **do**
    $\alpha_k = \frac{\mathbf{r}_k^{\mathsf{H}}\mathbf{r}_k}{\mathbf{p}_k^{\mathsf{H}}\bar{\mathbf{A}}\mathbf{p}_k}$
    $\mathbf{x}_{k+1} = \mathbf{x}_k + \alpha_k\mathbf{p}_k$
    $\mathbf{r}_{k+1} = \mathbf{r}_k - \alpha_k\bar{\mathbf{A}}\mathbf{p}_k$
    $\beta_k = \frac{\mathbf{r}_{k+1}^{\mathsf{H}}\mathbf{r}_{k+1}}{\mathbf{r}_k^{\mathsf{H}}\mathbf{r}_k}$
    $\mathbf{p}_{k+1} = \mathbf{r}_{k+1} + \beta_k\mathbf{p}_k$
**end for**

In the implementation, for each reconstruction scheme, we estimate $\bar{\mathbf{A}}$ and $\bar{\mathbf{y}}$ given the respective $\bar{f}$. Then, we calculate the reconstructed image $\mathbf{x}^* = \bar{\mathbf{A}}^{-1}\bar{\mathbf{y}}$ using Conjugate Gradient. Next, we detail the estimation of $\bar{\mathbf{A}}$ and $\bar{\mathbf{y}}$ for both cases.

**Conventional reconstruction** The data consistency function $\bar{f}$ becomes:

$$\bar{f}(\mathbf{x}) = f(\mathbf{x}) = \frac{1}{2}\|\mathbf{A}\mathbf{x} - \mathbf{y}\|_2^2 \tag{S8}$$

We replace $\bar{f}$ in equation S6 and find the equivalent linear problem by finding $\mathbf{x}^*$ such that $\nabla\bar{f}(\mathbf{x}^*) + \nabla\bar{g}(\mathbf{x}^*) = \mathbf{0}$.

$$\begin{aligned} \mathbf{x}^* &= \underset{\mathbf{x}}{\operatorname{argmin}}\, \frac{1}{2}\|\mathbf{A}\mathbf{x} - \mathbf{y}\|_2^2 + \frac{\lambda}{2}\|\mathbf{x}\|_2^2 \\ &= \left(\mathbf{A}^{\mathsf{H}}\mathbf{A} + \lambda\mathbf{I}\right)^{-1}\left(\mathbf{A}^{\mathsf{H}}\mathbf{y}\right) \end{aligned} \tag{S9}$$

Therefore, matrix $\bar{\mathbf{A}}$ and vector $\bar{\mathbf{y}}$ are the following:

$$\bar{\mathbf{A}} = \mathbf{A}^{\mathsf{H}}\mathbf{A} + \lambda\mathbf{I} \tag{S10a}$$

$$\bar{\mathbf{y}} = \mathbf{A}^{\mathsf{H}}\mathbf{y} \tag{S10b}$$

**Sketched reconstruction** Analogously, the data consistency term becomes:

$$\bar{f}(\mathbf{x}) = f_{\mathbf{S}}(\mathbf{x}) = \frac{1}{2}\|\mathbf{A}_{\mathbf{S}}(\mathbf{x}-\mathbf{x}^0)\|_2^2 + \langle \mathbf{x}, \mathbf{A}^{\mathsf{H}}(\mathbf{A}\mathbf{x}^0 - \mathbf{y})\rangle, \tag{S11}$$

where $\mathbf{x}^0$ is an initial estimate, which in the case of the manuscript is the previous estimation $\mathbf{x}^t$. Similarly, we estimate the equivalent linear problem.

$$\begin{aligned} \mathbf{x}^* &= \underset{\mathbf{x}}{\operatorname{argmin}} \frac{1}{2}\|\mathbf{A}_{\mathbf{S}}(\mathbf{x}-\mathbf{x}^0)\|_2^2 + \langle \mathbf{x}, \mathbf{A}^{\mathsf{H}}(\mathbf{A}\mathbf{x}^0 - \mathbf{y})\rangle + \frac{\lambda}{2}\|\mathbf{x}\|_2^2 \\ &= \left(\mathbf{A}_{\mathbf{S}}{}^{\mathsf{H}}\mathbf{A}_{\mathbf{S}} + \lambda\mathbf{I}\right)^{-1}\left(\mathbf{A}_{\mathbf{S}}{}^{\mathsf{H}}\mathbf{A}_{\mathbf{S}}\mathbf{x}^0 - \mathbf{A}^{\mathsf{H}}(\mathbf{A}\mathbf{x}^0 - \mathbf{y})\right) \end{aligned} \tag{S12}$$

Therefore, matrix $\bar{\mathbf{A}}$ and vector $\bar{\mathbf{y}}$ are the following:

$$\bar{\mathbf{A}} = \mathbf{A}_{\mathbf{S}}{}^{\mathsf{H}}\mathbf{A}_{\mathbf{S}} + \lambda\mathbf{I} \tag{S13a}$$

$$\bar{\mathbf{y}} = \mathbf{A}_{\mathbf{S}}{}^{\mathsf{H}}\mathbf{A}_{\mathbf{S}}\mathbf{x}^0 - \mathbf{A}^{\mathsf{H}}(\mathbf{A}\mathbf{x}^t - \mathbf{y}) \tag{S13b}$$

## S2.2 $\ell_1$-Wavelets regularization

Similarly, we consider the following optimization problem for image reconstruction:

$$\mathbf{x}^* = \underset{\mathbf{x}}{\operatorname{argmin}}\, \bar{f}(\mathbf{x}) + \bar{g}(\mathbf{x}) \tag{S14}$$

$$\bar{g}(\mathbf{x}) = \lambda\|\Psi\mathbf{x}\|_1 \tag{S15}$$

where $\bar{f} : \mathbb{C}^D \to \mathbb{R}$ is the data consistency function and $\bar{g} : \mathbb{C}^D \to \mathbb{R}$ is the regularization function. The data consistency function is a quadratic term in both conventional and sketched reconstruction. In this case, since $\bar{g}(\mathbf{x})$ is non-smooth, our approach solves the optimization problem using the Fast Iterative Shrinkage-Thresholding Algorithm (FISTA) [35] as shown in Algorithm S2. In general, FISTA can efficiently solve optimization problems of the form of equation S14 when $\bar{f}$ is smooth, convex, and continuously differentiable with Lipschitz continuous gradient, and $\bar{g}$ is continuous convex and possibly non-smooth [35]. In both conventional and sketched reconstruction, the data consistency function $\bar{f}$ is a quadratic term and, thus, complies with the requirements.

In algorithm S2, $\nabla\bar{f}$ denotes the gradient of $\bar{f}$ and $\mathrm{prox}_{\alpha\bar{g}}$ denotes the proximal operator of $\bar{g}$ with parameter $\alpha$. Since the wavelets transform $\Psi$ is an orthonormal basis, the proximal operator can be efficiently computed as follows:

$$\mathrm{prox}_{\alpha\bar{g}}(\mathbf{x}) = \Psi^{\mathsf{H}}\mathcal{T}_{\alpha\lambda}(\Psi\mathbf{x}), \tag{S16}$$

where $\mathcal{T}_{\alpha\lambda}$ is the soft-thresholding operation with threshold $\alpha\lambda$.

In the implementation, for each reconstruction scheme, we estimate the respective $\nabla\bar{f}$. Then, we calculate the reconstructed image $\mathbf{x}^*$ using FISTA. Next, we detail the estimation of $\nabla\bar{f}$ for both cases.

**Algorithm S2** Fast Iterative Shrinkage-Thresholding Algorithm (FISTA)

**Input:** Functions $\bar{f}$ and $\bar{g}$, step size $\alpha$
**Output**: Reconstructed image $\mathbf{x}_K$
Initialize $\mathbf{x}_0$
$\beta_0 = 1$
$\mathbf{z}_0 = \mathbf{x}_0$
**for** $k = 0, ..., K-1$ **do**
  $\mathbf{x}_{k+1} = \text{prox}_{\alpha \bar{g}} \left( \mathbf{z}_k - \alpha \nabla \bar{f}(\mathbf{z}_k) \right)$
  $\beta_{k+1} = \frac{1+\sqrt{1+4\beta_k^2}}{2}$
  $\mathbf{z}_{k+1} = \mathbf{x}_{k+1} + \frac{\beta_k}{\beta_{k+1}} \left( \mathbf{x}_{k+1} - \mathbf{x}_k \right)$
**end for**

**Conventional reconstruction** The data consistency function $\bar{f}$ and its respective gradient $\nabla \bar{f}$ are shown below.

$$\bar{f}(\mathbf{x}) = f(\mathbf{x}) = \frac{1}{2} \|\mathbf{A}\mathbf{x} - \mathbf{y}\|_2^2 \tag{S17}$$

$$\nabla \bar{f}(\mathbf{x}) = \nabla f(\mathbf{x}) = \mathbf{A}^{\mathsf{H}}(\mathbf{A}\mathbf{x} - \mathbf{y}) \tag{S18}$$

**Sketched reconstruction** The data consistency function $\bar{f}$ and its respective gradient $\nabla \bar{f}$ are shown below.

$$\bar{f}(\mathbf{x}) = f_{\mathbf{S}}(\mathbf{x}) = \frac{1}{2} \|\mathbf{A}_{\mathbf{S}}(\mathbf{x} - \mathbf{x}^0)\|_2^2 + \langle \mathbf{x}, \mathbf{A}^{\mathsf{H}}(\mathbf{A}\mathbf{x}^0 - \mathbf{y}) \rangle \tag{S19}$$

$$\nabla \bar{f}(\mathbf{x}) = \nabla f_{\mathbf{S}}(\mathbf{x}) = {\mathbf{A}_{\mathbf{S}}}^{\mathsf{H}} \mathbf{A}_{\mathbf{S}}(\mathbf{x} - \mathbf{x}^0) + \mathbf{A}^{\mathsf{H}}(\mathbf{A}\mathbf{x}^0 - \mathbf{y}), \tag{S20}$$

where $\mathbf{x}^0$ is an initial estimate, which in the case of the manuscript is the previous estimation $\mathbf{x}^t$.

## S2.3 $\ell_1$-TV regularization

We consider the following optimization problem for image reconstruction:

$$\mathbf{x}^* = \underset{\mathbf{x}}{\text{argmin}} \, \bar{f}(\mathbf{x}) + \bar{g}(\mathbf{T}\mathbf{x}) \tag{S21}$$

$$\bar{g}(\mathbf{x}) = \lambda \|\mathbf{x}\|_1 \tag{S22}$$

where $\bar{f} : \mathbb{C}^D \to \mathbb{R}$ is the data consistency function, $\bar{g} : \mathbb{C}^D \to \mathbb{R}$ is the regularization function, and $\mathbf{T}$ is the Total Variation operator. The data consistency function is a quadratic term in both conventional and sketched reconstruction. In this case, since $\mathbf{T}$ is not an orthonormal basis, our approach uses the Primal Dual Hybrid Gradient (PDHG) from Chambolle and Pock [36] as shown in Algorithm S3. In general, PDHG can solve problem of the form of equation S21 when $\bar{f}$ and $\bar{g}$ are proper, convex, and lower-semicontinuous functions and $\mathbf{T}$ is a continuous linear operator.

In algorithm S3, $\text{prox}_{\alpha \bar{g}^*}$ denotes the proximal operator of the convex conjugate of $\bar{g}$ with parameter $\alpha$. This proximal operator has the closed-form solution shown in equation S23.

$$\begin{aligned} \text{prox}_{\sigma \bar{g}^*}(\mathbf{z}) &= \mathbf{z} - \sigma \text{prox}_{\frac{1}{\sigma} g}(\frac{1}{\sigma}\mathbf{z}) \\ &= \mathbf{z} - \sigma \mathcal{T}_{\frac{\lambda}{\sigma}}(\frac{1}{\sigma}\mathbf{z}) \end{aligned} \tag{S23}$$

**Algorithm S3** Primal Dual Hybrid Gradient (PDHG)

**Input:** Functions $\bar{f}$ and $\bar{g}$, step sizes $\sigma$ and $\tau$
**Output**: Reconstructed image $\mathbf{x}_K$
Initialize $\mathbf{x}_0$
Initialize $\mathbf{z}_0$
$\tilde{\mathbf{x}}_0 = \mathbf{x}_0$
**for** $k = 1, ..., K-1$ **do**
    $\mathbf{z}_{k+1} = \text{prox}_{\sigma \bar{g}^*}(\mathbf{z}_k + \sigma \mathbf{T} \tilde{\mathbf{x}}_k)$
    $\mathbf{x}_{k+1} = \text{prox}_{\tau \bar{f}}\left(\mathbf{x}_k - \tau \mathbf{T}^{\mathsf{H}} \mathbf{z}_{k+1}\right)$
    $\tilde{\mathbf{x}}_{k+1} = \mathbf{x}_{k+1} + \theta(\mathbf{x}_{k+1} - \mathbf{x}_k)$
**end for**

Likewise, $\text{prox}_{\tau \bar{f}}$ denotes the proximal operator of $\bar{f}$ with parameter $\tau$ defined in equation S24.

$$\text{prox}_{\tau \bar{f}}(\mathbf{x}) = \underset{\mathbf{u}}{\text{argmin}}\, \bar{f}(\mathbf{u}) + \frac{1}{2\tau}\|\mathbf{u} - \mathbf{x}\|_2^2 \tag{S24}$$

Since $\bar{f}$ is a quadratic function in both reconstruction schemes, $\text{prox}_{\tau \bar{f}}$ will have equivalent linear problem forms solvable with Conjugate Gradient. Next, we detail the estimation of the linear forms.

**Conventional reconstruction** The proximal operator of $\bar{f}$ has the following equivalent linear form.

$$\begin{aligned} \text{prox}_{\tau \bar{f}}(\mathbf{x}) &= \text{prox}_{\tau f}(\mathbf{x}) \\ &= \underset{\mathbf{u}}{\text{argmin}}\, \frac{1}{2}\|\mathbf{A}\mathbf{u} - \mathbf{y}\|_2^2 + \frac{1}{2\tau}\|\mathbf{u} - \mathbf{x}\|_2^2 \\ &= \left(\mathbf{A}^{\mathsf{H}}\mathbf{A} + \frac{1}{\tau}\mathbf{I}\right)^{-1} \left(\mathbf{A}^{\mathsf{H}}\mathbf{y} + \mathbf{x}\right) \end{aligned} \tag{S25}$$

Therefore, matrix $\bar{\mathbf{A}}$ and vector $\bar{\mathbf{y}}$ are shown in equation S26 and the proximal operator can be solved with Conjugate Gradient.

$$\bar{\mathbf{A}} = \mathbf{A}^{\mathsf{H}}\mathbf{A} + \frac{1}{\tau}\mathbf{I} \tag{S26a}$$

$$\bar{\mathbf{y}} = \mathbf{A}^{\mathsf{H}}\mathbf{y} + \mathbf{x} \tag{S26b}$$

**Sketched reconstruction** The proximal operator of $\bar{f}$ has the following equivalent linear form.

$$\begin{aligned} \text{prox}_{\tau \bar{f}}(\mathbf{x}) &= \text{prox}_{\tau f_{\mathbf{S}}}(\mathbf{x}) \\ &= \underset{\mathbf{u}}{\text{argmin}}\, \frac{1}{2}\|\mathbf{A}_{\mathbf{S}}(\mathbf{u} - \mathbf{x}^0)\|_2^2 + \langle \mathbf{x}, \mathbf{A}^{\mathsf{H}}(\mathbf{A}\mathbf{x}^0 - \mathbf{y})\rangle + \frac{1}{2\tau}\|\mathbf{u} - \mathbf{x}\|_2^2 \\ &= \left({\mathbf{A}_{\mathbf{S}}}^{\mathsf{H}}\mathbf{A}_{\mathbf{S}} + \frac{1}{\tau}\mathbf{I}\right)^{-1} \left({\mathbf{A}_{\mathbf{S}}}^{\mathsf{H}}\mathbf{A}_{\mathbf{S}}\mathbf{x}^0 - \mathbf{A}^{\mathsf{H}}(\mathbf{A}\mathbf{x}^0 - \mathbf{y}) + \mathbf{x}\right) \end{aligned} \tag{S27}$$

Therefore, matrix $\bar{\mathbf{A}}$ and vector $\bar{\mathbf{y}}$ are shown in equation S28 and the proximal operator can be solved with Conjugate Gradient.

$$\bar{\mathbf{A}} = \mathbf{A_S}^{\mathsf{H}}\mathbf{A_S} + \frac{1}{\tau}\mathbf{I} \tag{S28a}$$

$$\bar{\mathbf{y}} = \mathbf{A_S}^{\mathsf{H}}\mathbf{A_S}\mathbf{x}^0 - \mathbf{A}^{\mathsf{H}}(\mathbf{A}\mathbf{x}^0 - \mathbf{y}) + \mathbf{x} \tag{S28b}$$

## S3 Figures

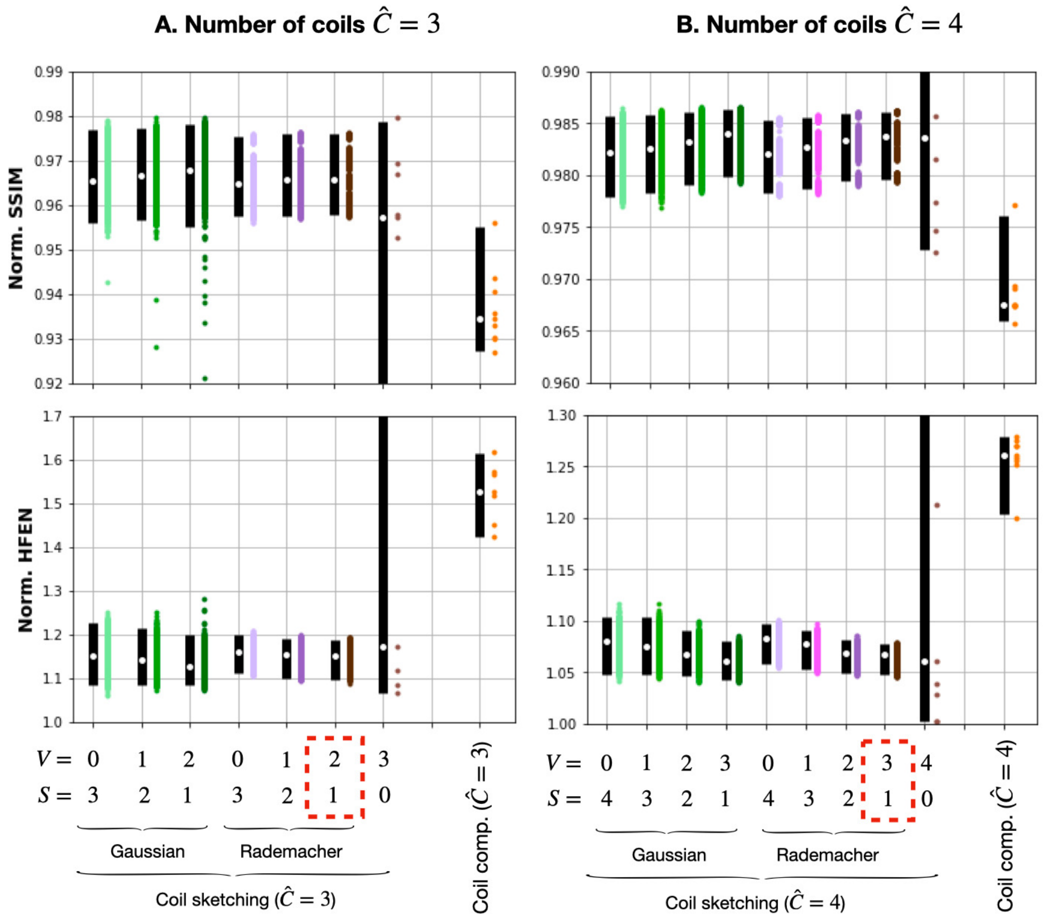


Figure S1: Evaluation of sketching matrix design through normalized SSIM and normalized HFEN for $\ell_1$-Wavelets reconstruction with 2D radial dataset. We report results for reduced number of coils **(A)** $\hat{C} = 3$ and **(B)** $\hat{C} = 4$. Similarly to Figure 2, Rademacher distribution shows increased precision when compared to Gaussian distribution. Furthermore, reconstruction accuracy is improved by increasing the number of virtual coils $V$ up to $V = \hat{C} - 1$

.

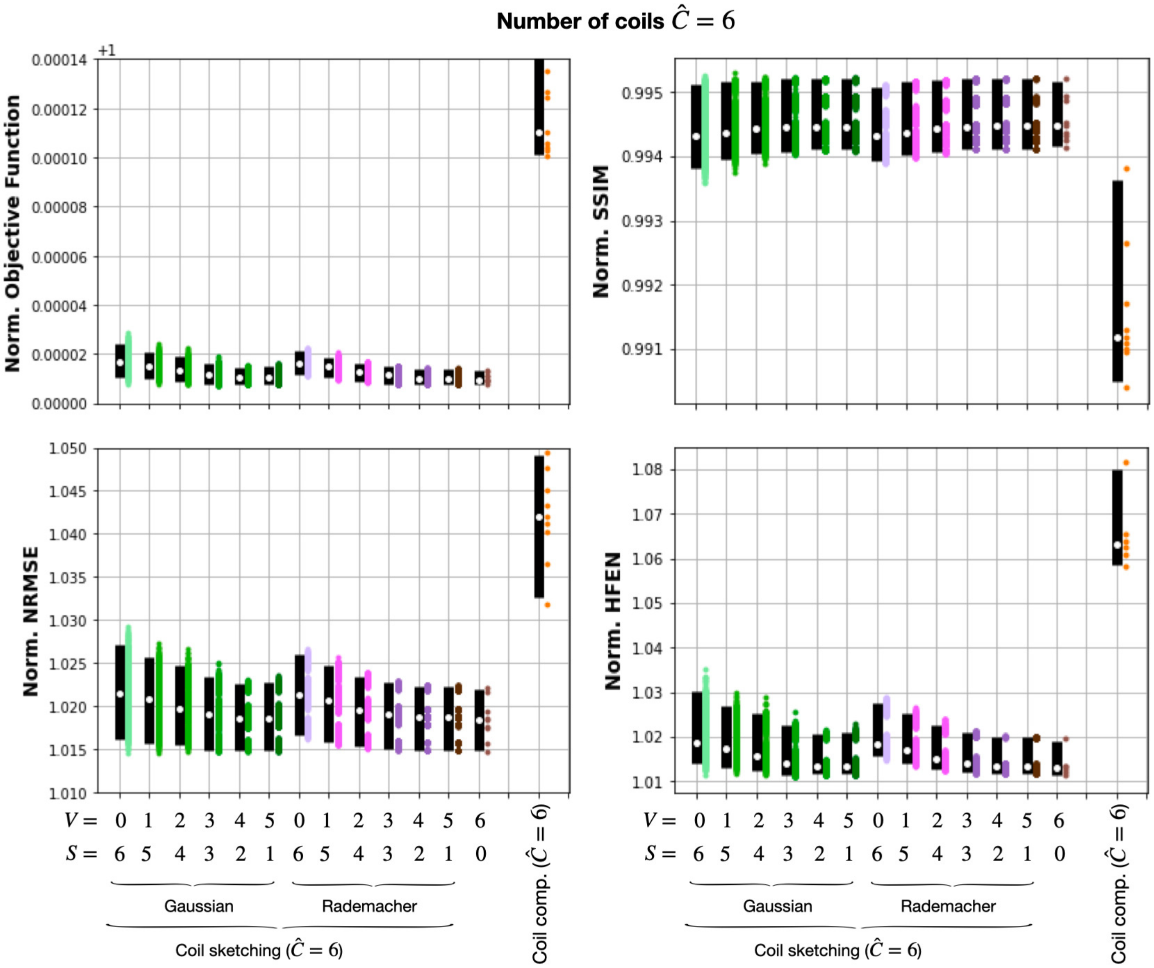


Figure S2: Evaluation of sketching matrix design through objective function value and image quality metrics for $\ell_1$-Wavelets reconstruction with 2D radial dataset. For a high number of coils $\hat{C} = 6$, out of $C = 8$ coils, reconstruction with $V = \hat{C}$ is no longer unstable and yields acceptable reconstructions. We hypothesize that the high number of coils ($\hat{C} = 6$) used with the iterative hessian sketch formulation yields an effective approximation that is able to perform correct reconstructions.

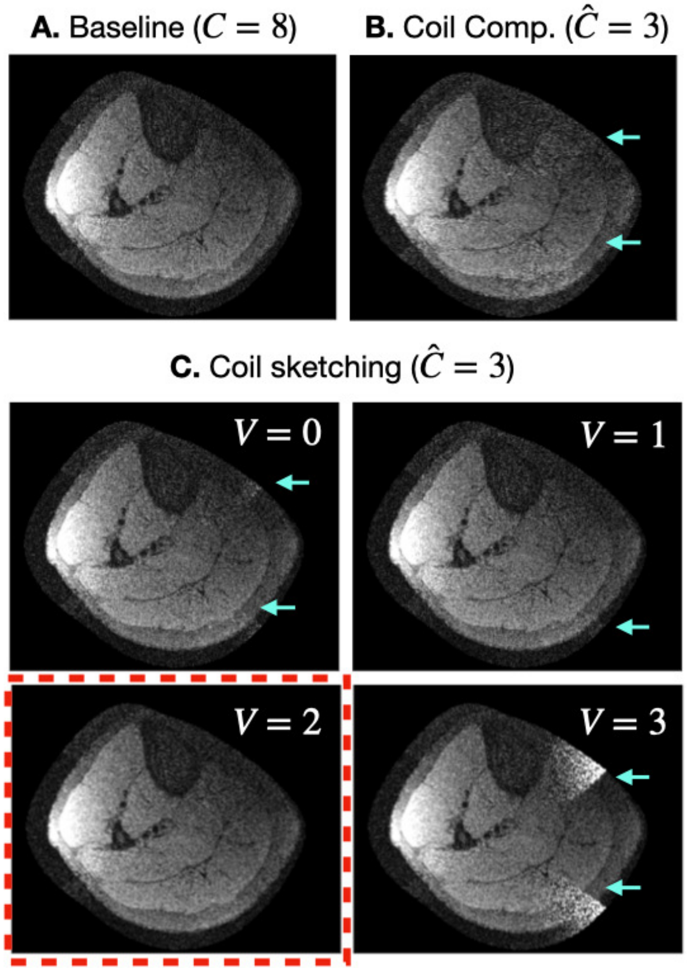


Figure S3: Exemplary reconstructed images from inverse g-factor experiment. Regions with lower inverse g-factor correspond to regions with increased noise.

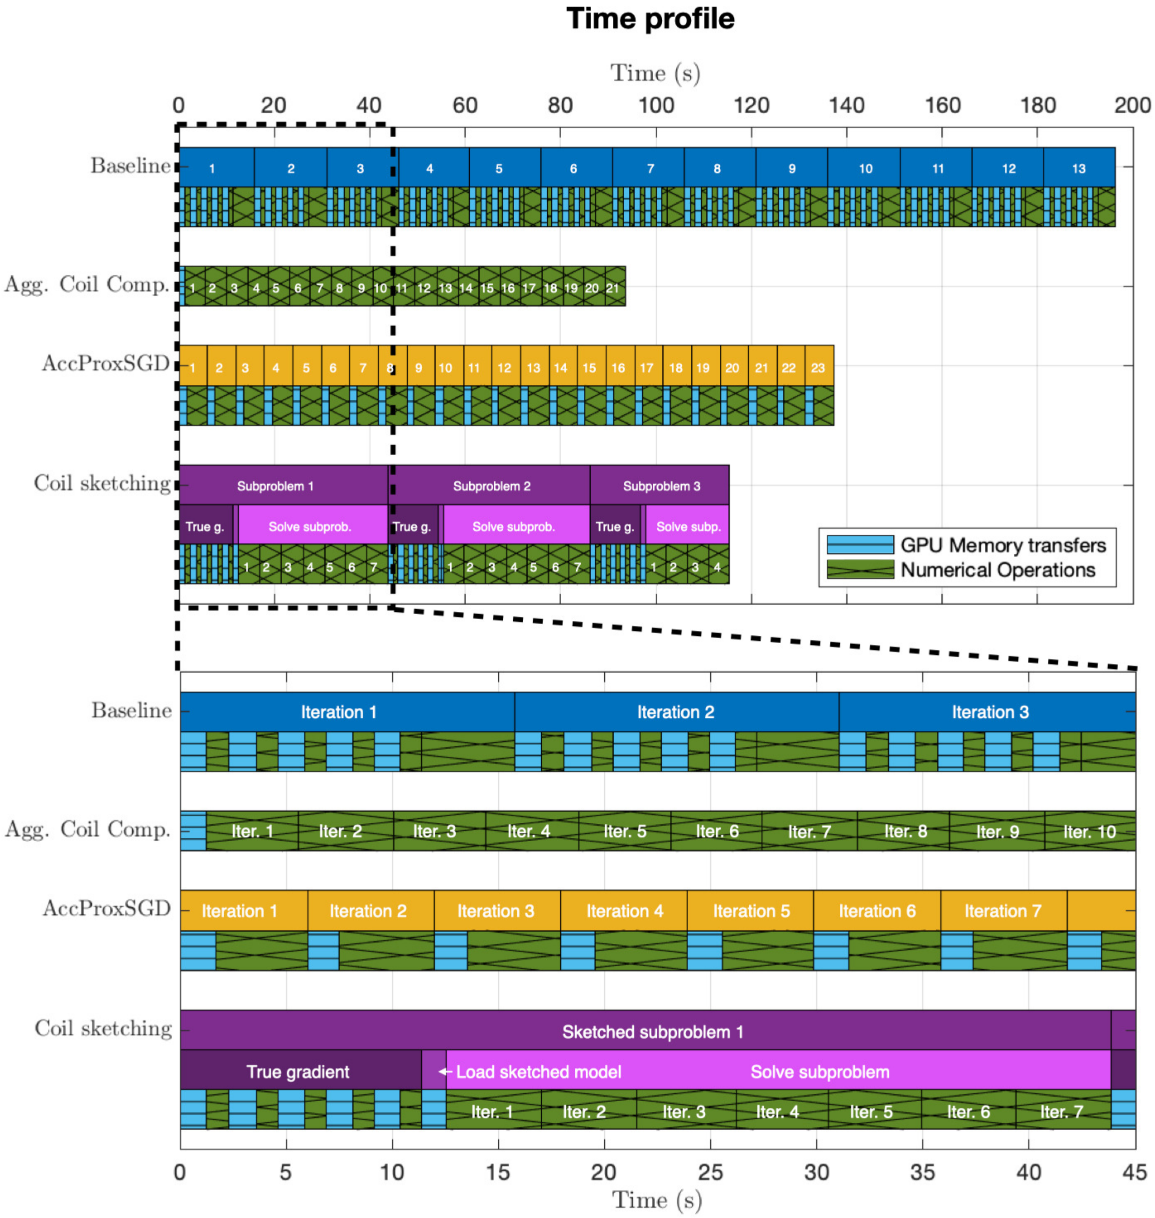


Figure S4: Time profile of the $\ell_1$-Wavelets experiment. Sky blue segments correspond to GPU memory transfers, i.e. loading/unloading coil sensitivity maps, whereas green segments correspond to numerical operations such as FFTs, Wavelets transforms, and soft-thresholding.
